# Supplementary material for: Plug-and-Play Multi-Concept Adaptive Blending for High-Fidelity Text-to-Image Synthesis
Source: arXiv:2511.17615 source file (2025-11-18)
Supplement: Supplementary file 1 [file appendices.tex]

% \input{chapters/appendix_codes}
