# Supplementary material for: Plug-and-Play Multi-Concept Adaptive Blending for High-Fidelity Text-to-Image Synthesis
Source: arXiv:2511.17615 source file (2025-11-18)
Supplement: Supplementary file 2 [file appendix_codes.tex]

% \chapter{Python Codes}

% Our demonstration has been conducted in a python environment.
% The following python codes execute the message updates and decision process. 
% Note that this is abstract information for the implementation of SP algorithm and other functions such as weight(partial sum rate) generator are required for the simulation.\\[1em]

% \begin{lstlisting}[language=Python]
% import numpy as np

% # x: state vector, x_j0: state of preallocated user

% def configurations(dim_x, n_pilot, neighbor_mapping, x_j0):
%     map_neighbor = np.zeros((dim_x, dim_x), dtype=int)
%     j0_prime = np.zeros((dim_x, dim_x, dim_x), dtype=int)
%     j0_window = np.zeros((dim_x, dim_x, n_pilot), dtype=int)
%     for i in range(dim_x):
%         neighbor_mapping[i, neighbor_mapping[i]] = 1
%         j0_window[i, x_j0[i], :] = 1
%         for j0 in x_j0[i]:
%             j0_prime = list(set(neighbor_mapping[j0]) - set(neighbor_mapping[i]))
%             j0_prime[i, j0, j0_prime] = 1
%     j_prime = np.tile(neighbor_mapping, (dim_x, 1, 1))
%     col_window = 1 - np.tile(np.expand_dims(np.eye(dim_x, dtype=int), axis=1), (1, dim_x, 1))
%     j_prime[col_window==0] = 0
%     row_window = 1 - np.tile(np.expand_dims(np.eye(dim_x), axis=2), n_pilot)
%     return neighbor_mapping, j_prime, j0_prime, row_window, j0_window

% # R: matrix of partial sum-rates
% # rT: rT, rB: rB
% # aT: aT, aB: aB

% def update_rho(R, aT_now, aB_now):
%     dim_x, n_pilot = np.shape(R)
%     rB_now = np.zeros(shape=(dim_x, n_pilot))
%     rT_now = np.zeros(shape=(dim_x, n_pilot))
%     for r in range(n_pilot):
%         aT_except_r = np.delete(aT_now, r, axis=1)
%         aB_except_r = np.delete(aB_now, r, axis=1)
%         R_except_r = np.delete(R, r, axis=1)
%         rT_now[:, r] = R[:, r] + np.sum(
%             aT_except_r - aB_except_r, axis=1)
%         rB_now[:, r] = R[:, r] - np.max(
%             R_except_r + aB_except_r, axis=1)
%     return rT_now, rB_now


% def update_alpha(map_neighbor, j_prime, j0_prime,
%                  row_window, j0_window, rT_now, rB_now):
%     dim_x, _ = np.shape(rT_now)
%     diff_rBT_n = np.minimum(rB_now - rT_now, 0)
%     diff_rBT_p = np.maximum(rB_now - rT_now, 0)
%     rB_tile = np.tile(rB_now, (dim_x, 1, 1))
%     diff_rBT_p_tile = np.tile(diff_rBT_p, (dim_x, 1, 1))
%     diff_rBT_n_tile = np.tile(diff_rBT_n, (dim_x, 1, 1))
%     j_prime_term_tile = np.matmul(j_prime, diff_rBT_n_tile)
%     j0_prime_term_tile = np.matmul(j0_prime, diff_rBT_n_tile)
    
%     term1 = np.matmul(map_neighbor, diff_rBT_n)
%     term2 = -rB_tile + diff_rBT_p_tile - j_prime_term_tile
%     term2[row_window==0] = INFIN
%     aT_next = term1 + np.minimum(np.min(term2, axis=1), 0)
    
%     term3 = -rB_tile + diff_rBT_p_tile - j0_prime_term_tile
%     term3[j0_window==0] = INFIN
%     aB_next = np.minimum(np.min(term3, axis=1), 0)

%     return aT_next, aB_next


% def make_decision(x, aT_now, aB_now,
%                   rT_now, rB_now):
%     dim_x = len(x)
%     dim_r = np.size(aT_now, axis=1)
%     allocation = np.zeros(dim_x)

%     b_tilde = aT_now + rT_now
%     b_bar = aB_now + rB_now
%     for i in range(dim_x):
%         if np.max(b_tilde[i, :]) > 0:
%             allocation[i] = np.argmax(b_bar[i, :])
%         else:
%             allocation[i] = None
%     for r in range(dim_r):
%         if np.count_nonzero(allocation==r) == 0:
%             i_argmax = np.argmax(b_tilde[:, r])
%             allocation[i_argmax] = r
%     return allocation
    
% \end{lstlisting}
